# Supplementary material for: Measuring memorization in language models via probabilistic extraction
Source: arXiv:2410.19482 source file (2025-03-20)
Supplement: Supplementary file 1 [file appendix.tex]

\clearpage
\section{Comparison over extraction rates under different sampling schemes}\label{sec:sampling_schemes}
% \jamie{MOVE TO APPENDIX}

\begin{figure*}[t]
\captionsetup[subfigure]{justification=centering}
  \centering
\begin{subfigure}[t]{0.33\textwidth}
\centering
    \includegraphics[width=1.\linewidth]{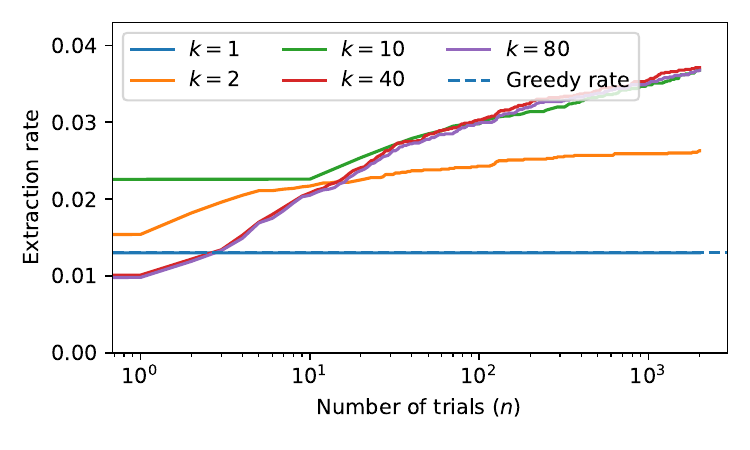}
        \caption{top-$k$, $p=10\%$.}
        \label{fig: topkp01}
\end{subfigure}%
\begin{subfigure}[t]{0.33\textwidth}
\centering
    \includegraphics[width=1.\linewidth]{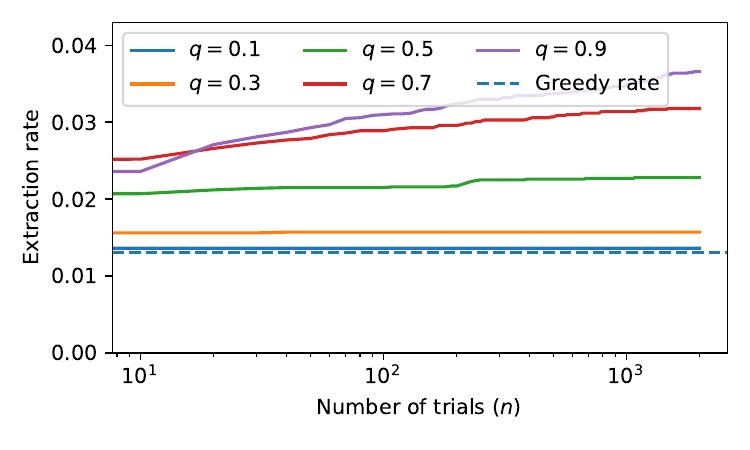}
        \caption{top-$q$, $p=10\%$.}
        \label{fig: toppp01}
\end{subfigure}%
\begin{subfigure}[t]{0.33\textwidth}
\centering
    \includegraphics[width=1.\linewidth]{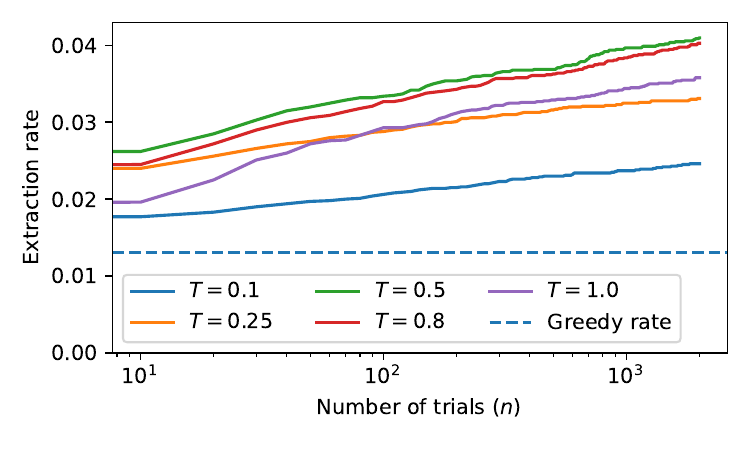}
        \caption{temperature ($T$), $p=10\%$.}
        \label{fig: tempt01}
\end{subfigure}
\begin{subfigure}[t]{0.33\textwidth}
\centering
    \includegraphics[width=1.\linewidth]{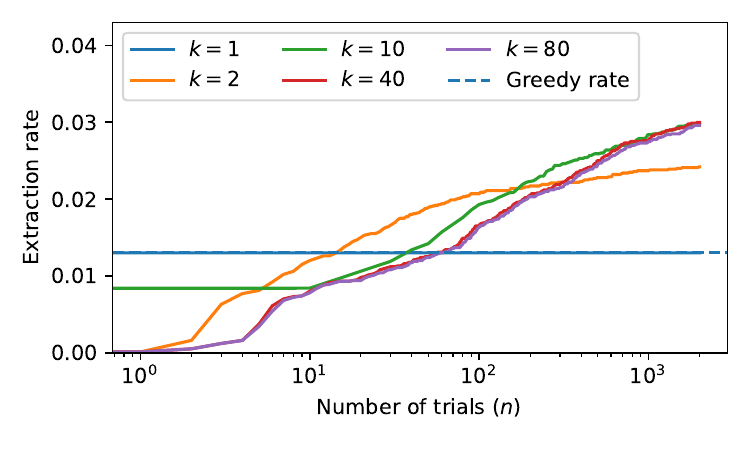}
        \caption{top-$k$, $p=90\%$.}
        \label{fig: topkp09}
\end{subfigure}%
\begin{subfigure}[t]{0.33\textwidth}
\centering
    \includegraphics[width=1.\linewidth]{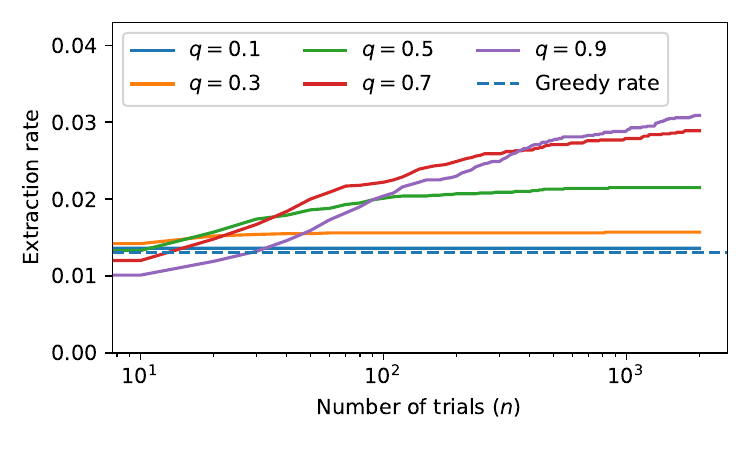}
        \caption{top-$q$, $p=90\%$.}
        \label{fig: toppp09}
\end{subfigure}%
\begin{subfigure}[t]{0.33\textwidth}
\centering
    \includegraphics[width=1.\linewidth]{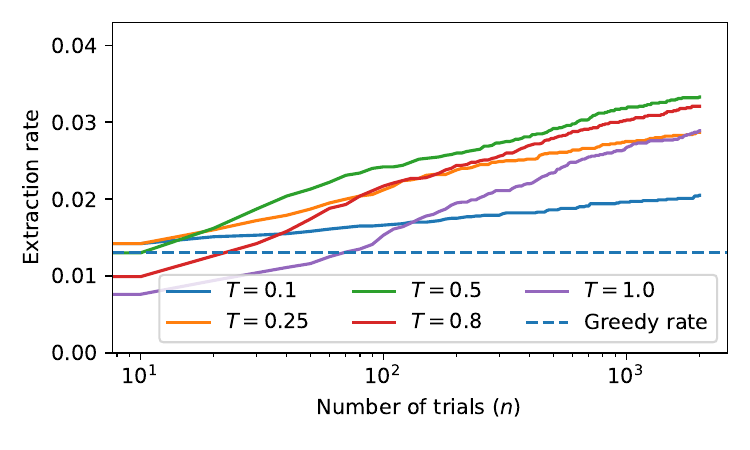}
        \caption{temperature ($T$), $p=90\%$.}
        \label{fig: tempt09}
\end{subfigure}%
\caption{Comparison of $(n, p)$-discoverable extraction rates for different sampling schemes. We fix $p$ to either 10\% or 90\%. In \Cref{fig: topkp01} and \Cref{fig: topkp09} we vary $k$ in top-$k$ sampling, in \Cref{fig: toppp01} and \Cref{fig: toppp09} we vary $q$ in top-$q$ sampling, and in \Cref{fig: tempt01} and \Cref{fig: tempt09} we vary $T$ in temperature sampling. Generally, smaller $k$, $q$ and $T$ confer smaller extraction rates, but is dependent on both $n$ and $p$. However, for most values and for small $n$, the extraction rate is above the greedy sampling based extraction rate.}
\label{fig: sampling_schemes}
\end{figure*}

We compare extraction rates under different choices of $n$ and $p$ using different sampling schemes. 
We perform additional experiments for top-$k$ and sampling with different temperatures (see \Cref{sec:prelim:sampling}).
We also include results for \textbf{nucleus sampling}, which we refer to as \textbf{top-$q$ sampling}. 
This is similar to top-$k$ sampling, but instead of keeping only the top-$k$ token probabilities, we  retain (and normalize) the smallest subset of tokens such that their cumulative probability is at least $q\in(0, 1]$. 
(Note that, in the literature, this is typically referred to as top-$p$ sampling; we relabel this as top-$q$ sampling to disambiguate with our use of $p$ in $(n,p)$-discoverable extraction.)

The results are summarized in \Cref{fig: sampling_schemes}, where we vary the sampling scheme specific hyperparameters $k$, $q$, and $T$, respectively. 
We make the following observations.
Firstly, in top-$k$ sampling, increasing $k$ can substantially increase extraction rates even for small $n$, and this effect becomes more pronounced with small values of $p$.
For example, in \Cref{fig: topkp01} where we fix $p=10\%$, the extraction rate at $k=2$ is $1.5\%$ at $n=1$; significantly higher than at $k=1$, and this difference only increases with $n$.
The same effect can be observed in \Cref{fig: topkp09} where we fix $p=90\%$, however at smaller $n$ ($n<20$) the difference is smaller.
In general, larger values of $k$ confer larger extraction rates, but this is affected by both $p$ and $n$; for small $p$, extraction rates for small $k$ are dominated by larger $k$, while for larger $p$, extraction rates for small $k$ dominate larger $k$, but this eventually reverses when $n$ becomes larger enough.
Similar trends can be observed for top-$q$ sampling, in \Cref{fig: toppp01} and \Cref{fig: toppp09}, and for temperature sampling in \Cref{fig: tempt01} and \Cref{fig: tempt09}, where larger values of $q$ and $T$, results in larger extraction rates as $n$ increases.

At first glance, one may wonder why there isn't a strict ordering of extraction rates for top-$k$, top-$q$, and temperature sampling, if rates are compared according scaling $k$, $q$, and $T$, respectively. 
$(n, p)$-discoverable extraction is designed such that expected extraction rate matches the amount of memorization emitted when an end user interacts with the model.
However, this is challenging as users are generally free to choose the underlying sampling scheme.
If we report a extraction rate under a choice of temperature $T$ and an end user choose to use a different temperature $T'\neq T$, is the reported extraction rate still useful?
The added complication here being that as $k$, $q$, or $T$ is varied, token probabilities can either increase or decrease. 
For example in top-$k$ sampling, as $k$ increases, the probability of sampling a specific token $z_i$ can either decrease (a larger $k$ results in more tokens available for sampling, decreasing the probability of sampling $z_i$) or increase (if at smaller $k$, $z_i$ had zero probability). 
This means $(n, p)$ extraction rates are not properly ordered according to the choice of $k$, $q$, or $T$. 
If a practitioner is concerned about the varying extraction rates under different sampling hyperparameters, it is easy to compute rates over different choices as we have done in \Cref{fig: sampling_schemes}.
Because top-$k$, top-$q$, and temperature sampling are post processing functions applied on top of the generated logit distribution over tokens, it is extremely cheap to compute these rates over different sampling hyperparameters.

% Fortunately, the answer is yes, as under the same sampling scheme, there is a positive correlation between the probability of a sequence and reducing (or increasing) the sampling scheme hyperparameter that controls the amount of randomness introduced into sampling the next token.
% Firstly, the probability of sampling a specific token

% [0.4, 0.3, 0.2, 0.1]
% [0.4, 0.3, 0.1, 0]
% []

% We deal with the three most common random sampling scheme individually: top-$k$, top-$q$, and random (under temperature T), and show empirically that we can bound and accurately infer the amount of memorization under different choices of sampling hyperparameter.

% \noindent \textit{top-k and top-p} \jamie{We can bound this!! i.e. probability of generating a sample will only go down BUT more examples can appear as smaller k will cutoff examples more than larger k!!} \itay{Recently people started advocating min-p sampling: https://arxiv.org/abs/2407.01082, it actually might be more leaking then the three most common aforementioned.}

% \noindent \textit{Temperature T}  \jamie{We can collect the original prob dist and then apply as post processing, cheap to get results! We can also bound}

% \jamie{in in \Cref{fig: topkp01} explain why things aren't well ordered}

\section{Additional discussion of related definitions}\label{app:sec:othermem}

\section{Extraction rates for repeated training data}\label{sec: nonlog_rep}

\begin{figure}[H]
  \centering
    \includegraphics[width=1.0\linewidth]{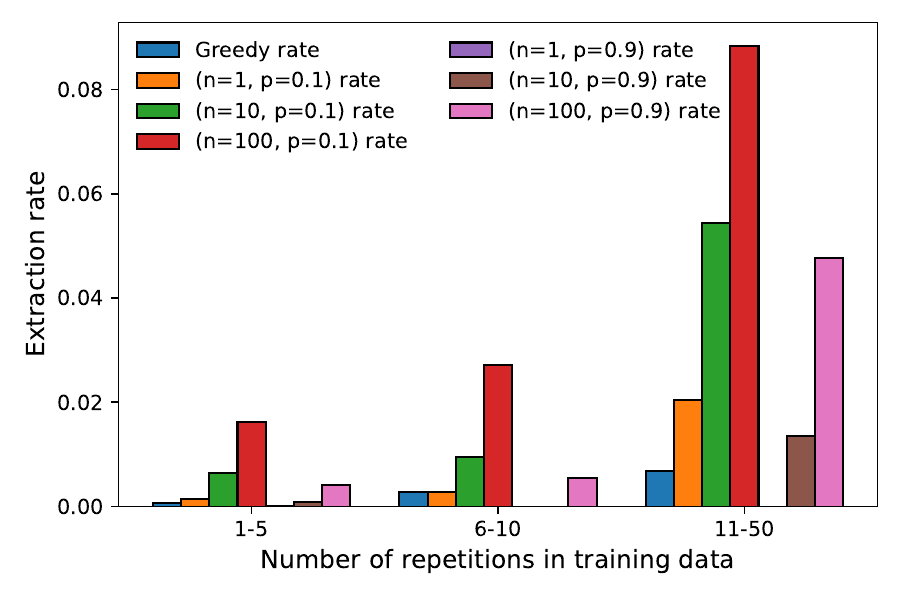}
  \caption{We plot a non log scale version of \Cref{fig: topk2b_rep_data} to make it clear that the difference between the greedy sampling extraction rate and $(n, p)$ rate increases with more training data repetitions.}
\label{fig: topk2b_rep_data_no_log}
\end{figure}

\section{Does the theoretical extraction rate match empirical results?}\label{sec:compare_theory}

% \begin{wrapfigure}{r}{0.5\textwidth}
%   \begin{center}
% \includegraphics[width=0.5\textwidth]{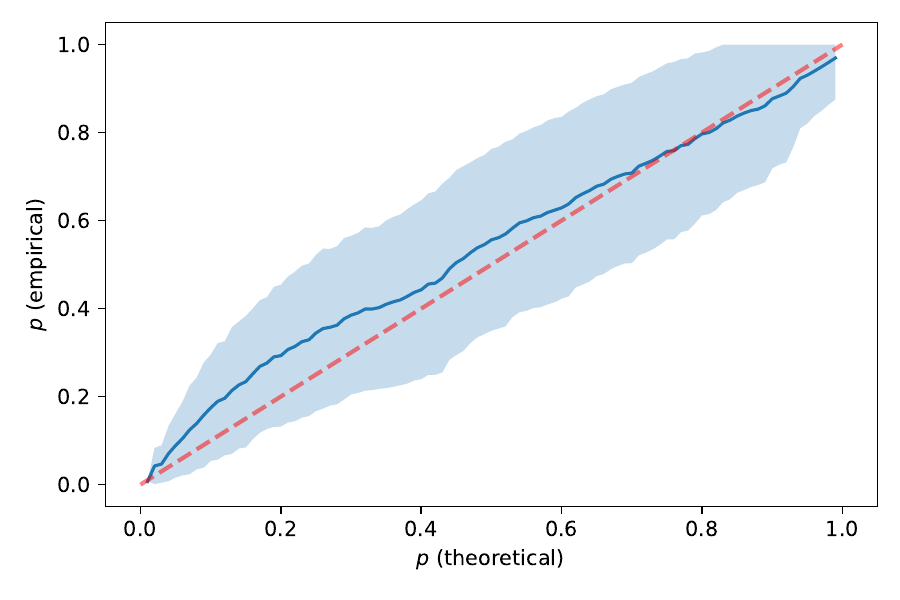}
%   \end{center}
%   \caption{We check that generating a set of $n$ sequences and checking the probability a training example appears at least once in the set (empirical $p$), matches the theoretical $p$ according to \Cref{eq:npmem}.}
%   \label{fig: emp_p}
% \end{wrapfigure}

\begin{figure}[H]
  \begin{center}
\includegraphics[width=1.0\linewidth]{figures/empirical_p.pdf}
  \end{center}
  \caption{We check that generating a set of $n$ sequences and checking the probability a training example appears at least once in the set (empirical $p$), matches the theoretical $p$ according to \Cref{eq:npmem}.}
  \label{fig: emp_p}
\end{figure}

So far, we have reported memorization found through \Cref{eq:npmem}.
This means for a given training example, we find the probability of generating the target suffix, and then for a fixed $p$, we find the corresponding $n$ according to \Cref{eq:npmem}.
Here, we confirm that this procedure aligns with the (more costly) empirical procedure of sampling $n$ sequences, and checking the probability that the sequence appears in the set is $p$.

For 1,000 training examples, and for a fixed $p$, we calculate the $n$ such that sampling $n$ sequences should result in a fraction of $p$ matches. 
For each training example, we then generate $n$ sequences and check if the example appears in the set.
We then check if a fraction $p$ of the examples did appear in their associated sets, over the 1,000 examples. 
Results are given in \Cref{fig: emp_p}, showing expected $p$ according to our theory does match the empirical calculated $p$.

\section{Distribution of perplexity scores}

\begin{figure*}[t]
\captionsetup[subfigure]{justification=centering}
 \captionsetup[subfigure]{width=0.9\textwidth}
  \centering
\begin{subfigure}[t]{0.33\textwidth}
\centering
    \includegraphics[width=0.95\linewidth]{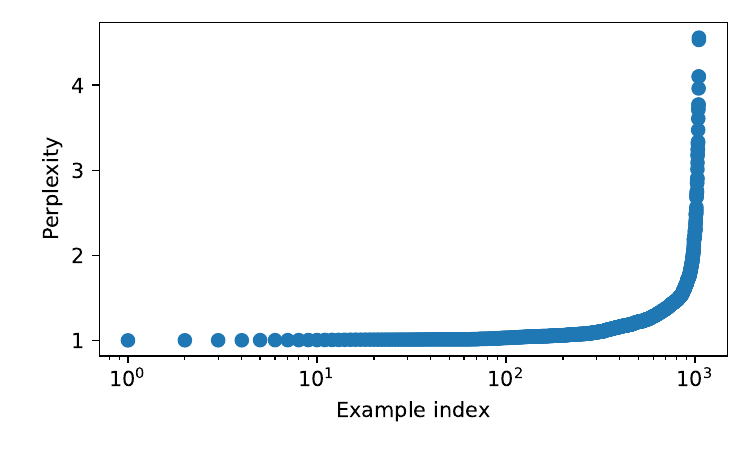}
        \caption{Perplexity scores for target suffixes with top-$k=40$.}
        \label{fig: ppxtopk}
\end{subfigure}%
\begin{subfigure}[t]{0.33\textwidth}
\centering
    \includegraphics[width=0.95\linewidth]{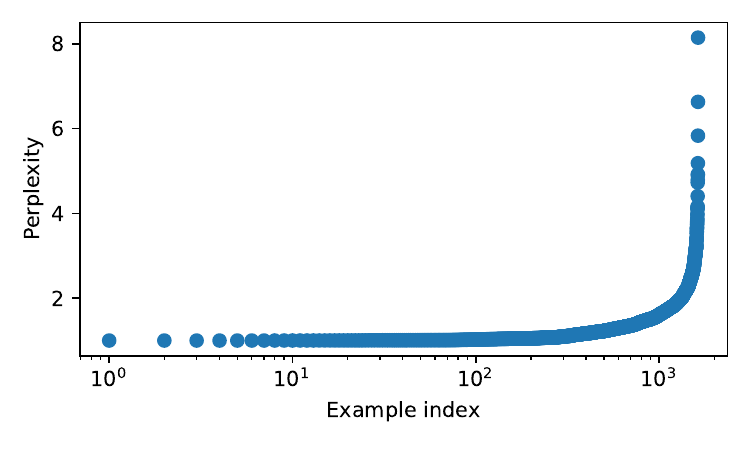}
        \caption{Perplexity scores for target suffixes with top-$q=0.9$.}
        \label{fig: ppxtopq}
\end{subfigure}%
\begin{subfigure}[t]{0.33\textwidth}
\centering
    \includegraphics[width=0.95\linewidth]{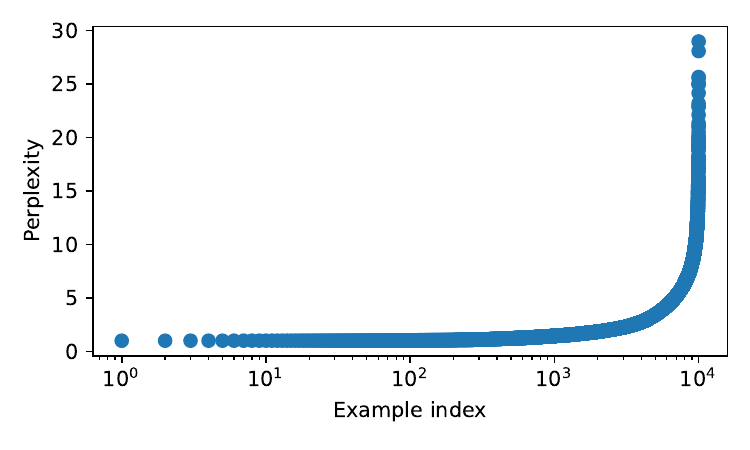}
        \caption{Perplexity scores for target suffixes with random sampling with $T=1$.}
        \label{fig: ppxt}
\end{subfigure}
\begin{subfigure}[t]{0.33\textwidth}
\centering
    \includegraphics[width=0.95\linewidth]{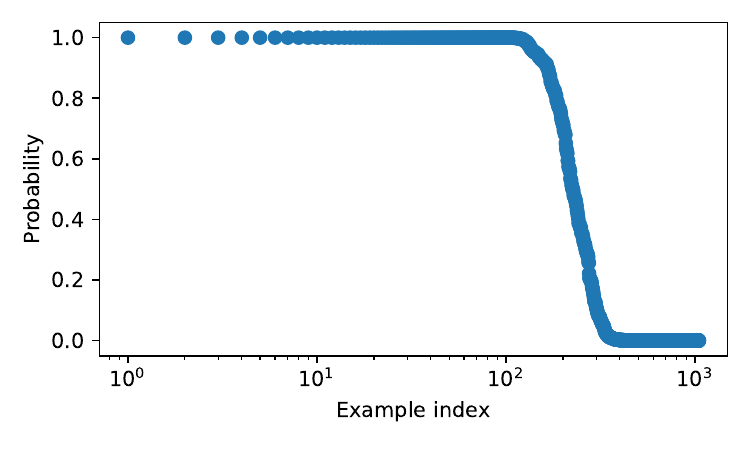}
        \caption{Probability of sampling the target suffix within $n=100$ trials for top-$k=40$ sampling.}
        \label{fig: probtopk}
\end{subfigure}%
\begin{subfigure}[t]{0.33\textwidth}
\centering
   \includegraphics[width=0.95\linewidth]{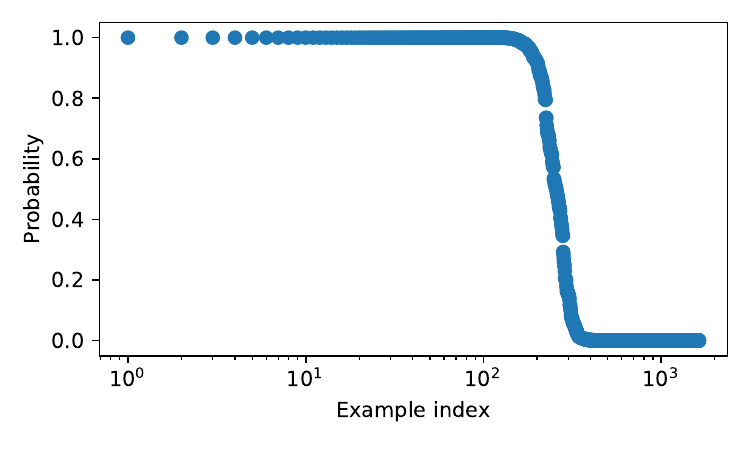}
        \caption{Probability of sampling the target suffix within $n=100$ trials for top-$q=0.9$ sampling.}
        \label{fig: probtopq}
\end{subfigure}%
\begin{subfigure}[t]{0.33\textwidth}
\centering
    \includegraphics[width=0.95\linewidth]{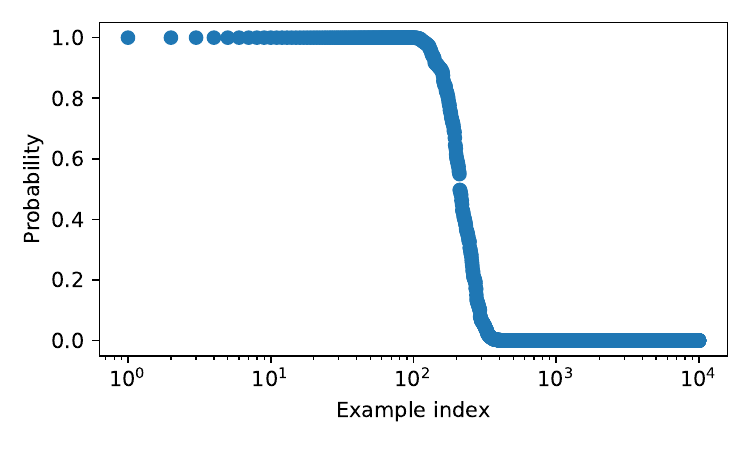}
        \caption{Probability of sampling the target suffix within $n=100$ trials for random sampling with $T=1$.}
        \label{fig: probt}
\end{subfigure}
\caption{For each of the 10,000 Enron examples, we plot the perplexity score of the target suffix for a choice of sampling scheme. We also plot the probability that each of the target suffixes will be sampled within $n=100$ trials. Note, for top-$k$ and top-$q$ sampling, there are fewer than 10,000 examples plotted. This is because many target suffixes have a zero probability of being sampled under the sampling scheme.}
\label{fig: ppxandprob}
\end{figure*}

For each of the 10,000 Enron examples, we plot the perplexity score of the target suffix for a choice of sampling scheme (top-$k=40$, top-$q=0.9$, random sampling with $T=1$) in \Cref{fig: ppxtopk,fig: ppxtopq,fig: ppxt}.
For reference, we also plot the probability that each of the target suffixes will be sampled within $n=100$ trials in \Cref{fig: probtopk,fig: probtopq,fig: probt}.

From \Cref{fig: ppxtopk}, we see that nearly 9,000 examples do not have a perplexity score. 
This is because it was impossible to sample the target suffix with top-$k=40$ sampling, because at least one of the tokens in the sequence has a zero probability of being sampled.
Out of the 1,000 suffixes that could be sampled successfully, the majority have extremely low perplexity.
This is reflected in \Cref{fig: probtopk}, where we observe that the a large fraction of examples will almost certainly being sampled within $n=100$ trials.
A similar set of observations can be made for top-$q=0.9$ sampling in \Cref{fig: ppxtopq,fig: probtopq}.
For random sampling with $T=1$, in theory all possible sequences could be sampled, and so each of the 10,000 examples has a defined perplexity score. 
Again, we see that a large fraction of target suffix sequences have small perplexity scores; from \Cref{fig: probt}, approximately 250 target suffix examples will almost surely be sampled within $n=100$ trials.

\section{More examples of how greedy sampling can mask signs of memorization}\label{app: more_why}

% We include the text for the target and generated sequences omitted from Figure~\ref{fig: greedy_fail}.
% \begin{figure}[t]
%   \centering
%     \includegraphics[width=0.4\linewidth]{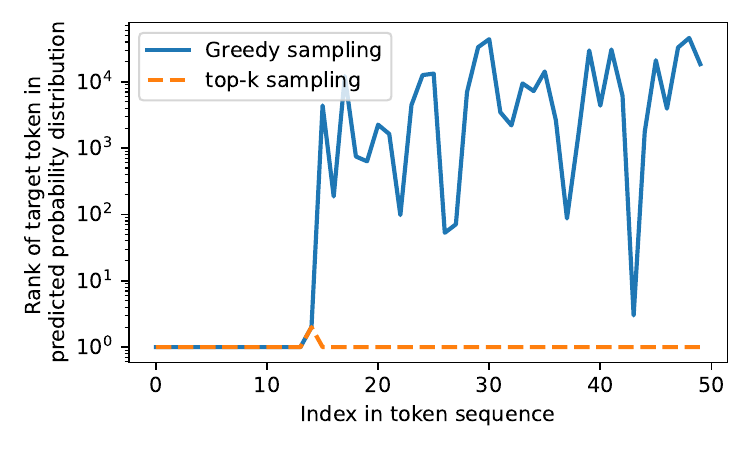}
%   \caption{\textbf{Prefix:} \textit{``\escape{n}\escape{n}The information contained herein is based on sources that we believe to be\escape{n}reliable, but we do not represent that it is accurate or complete.  Nothing\escape{n}contained herein should be considered as an offer to sell or a solicitation\escape{n}of an''}, \textbf{Suffix (predicted from greedy sampling):} \textit{`` offer to buy any financial instruments discussed herein.  Any\escape{n}opinions{\color{carminered}, estimates, or other information contained in this communication\escape{n}is solely the responsibility of the author.\escape{n} - att1.htm}''}. \textbf{Target Suffix:} \textit{`` offer to buy any financial instruments discussed herein.  Any\escape{n}opinions {\color{greenncs}  expressed herein are solely those of the author.  As such, they\escape{n}may differ in material respects from those of, or expressed or published by\escape{n}on behalf of Carr Futures}'', where we highlight the differences between {\color{carminered} predicted} and {\color{greenncs} target} tokens}. }
% \label{fig: greedy_fail_full}
% \end{figure}

Following from \Cref{fig: greedy_fail} and  \Cref{sec:def} we give three more of examples in \Cref{fig: examples} of cases where greedy sampling misses clear cases of memorization. We include the text for the target and generated sequences omitted from Figure~\ref{fig: greedy_fail}.

\begin{figure*}
  \centering
% \captionsetup{width=\linewidth} % This sets the caption width
\begin{subfigure}[t]{0.45\textwidth}
\centering
    \includegraphics[width=\linewidth]{figures/example_of_greedy_fail.pdf}
      \caption{\textbf{Prefix:} 
      {\footnotesize
      \textit{``\escape{n}\escape{n}The information contained herein is based on sources that we believe to be\escape{n}reliable, but we do not represent that it is accurate or complete.  Nothing\escape{n}contained herein should be considered as an offer to sell or a solicitation\escape{n}of an''}, \textbf{Suffix (predicted from greedy sampling):} \textit{`` offer to buy any financial instruments discussed herein.  Any\escape{n}opinions{\color{carminered}, estimates, or other information contained in this communication\escape{n}is solely the responsibility of the author.\escape{n} - att1.htm}''}. \textbf{Target Suffix:} \textit{`` offer to buy any financial instruments discussed herein.  Any\escape{n}opinions {\color{greenncs}  expressed herein are solely those of the author.  As such, they\escape{n}may differ in material respects from those of, or expressed or published by\escape{n}on behalf of Carr Futures}'', where we highlight the differences between {\color{carminered} predicted} and {\color{greenncs} target} tokens}. }}
    \label{fig: greedy_fail_full}
    \end{subfigure}\hfill
\begin{subfigure}[t]{0.45\textwidth}
\centering
    \includegraphics[width=\linewidth]{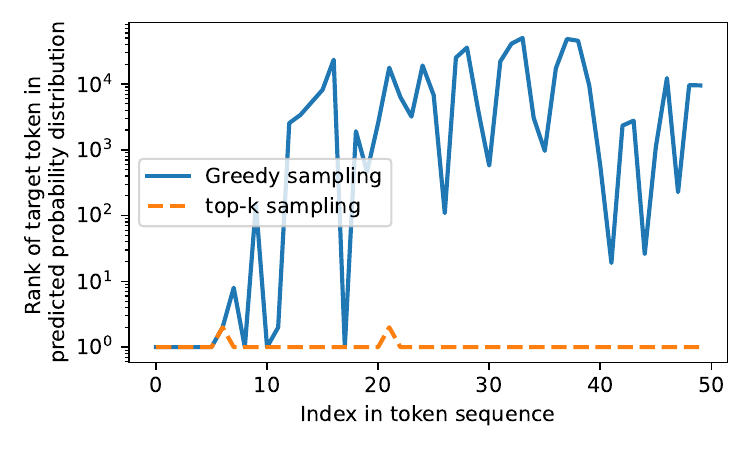}
        \captionsetup{width=\textwidth} % This sets the caption width
        \caption{
        {\footnotesize
        \textbf{Prefix: }\textit{``I do not.\escape{n}\escape{n} -----Original Message-----\escape{n}From: \escape{t}Panus, Stephanie  \escape{n}Sent:\escape{t}Monday, October 22, 2001 9:35 AM\escape{n}To:\escape{t}Bailey, Susan; Boyd, Samantha; Cook, Mary''}.
        \textbf{Suffix (predicted from greedy sampling): } \textit{``; ; Gray, Barbara N.; {\color{carminered} Greenberg, Mark; Hansen, Leslie; Heard, Marie; Hendry, Brent; Hodge, Jeffrey T.; Jones, Tana; Koehler, Anne C.; Leite, Francisco Pinto; Nelson}''}. \textbf{Target Suffix: } \textit{``; Gray, Barbara N.; {\color{greenncs} Heard, Marie; Hendry, Brent; Jones, Tana; Keiser, Holly; Koehler, Anne C.; Leite, Francisco Pinto; Nelson, Cheryl; Sayre, Frank;}''.}}}
        \label{fig: ex01}
\end{subfigure}
\begin{subfigure}[t]{0.45\textwidth}
\centering
    \includegraphics[width=\linewidth]{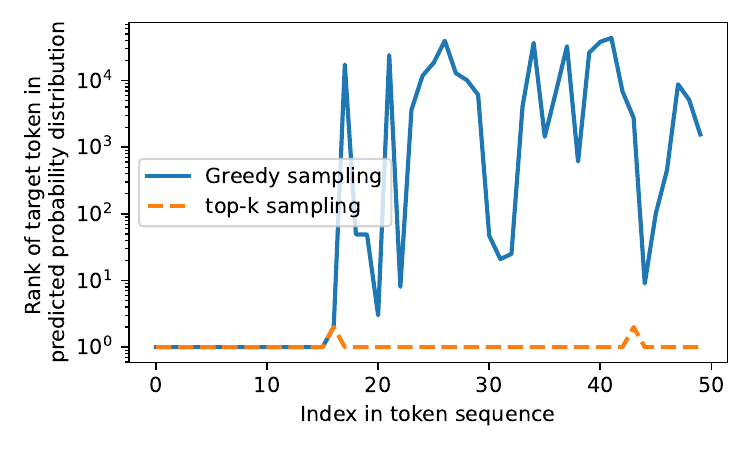}
        \captionsetup{width=\textwidth} % This sets the caption width
        \caption{
        {\footnotesize
        \textbf{Prefix: }\textit{``Version 2.0 of the ClickAtHome Portal is now available!  \escape{n}\escape{t}Log into www.clickathome.net now, from work or home!\escape{n}\escape{n}Access the PEP System through the portal!  \escape{n}\escape{t}Choose your reviewers''}.
        \textbf{Suffix (predicted from greedy sampling): } \textit{`` and fill out your evaluations in the comfort and privacy of your home!\escape{n}\escape{n}{\color{carminered}Your Portal Username:\escape{t}\escape{t}hgm3122\escape{n}Your Password:\escape{t}\escape{t}9hgm3122\escape{n}\escape{n}Welcome to PEP at http://www.click''}}. \textbf{Target Suffix: } \textit{`` and fill out your evaluations in the comfort and privacy of your home!\escape{n}\escape{n}{\color{greenncs}Outlook Web Access and eHRonline will be available SOON!  \escape{n}\escape{n}The ClickAtHome portal is fully customizable for you!  \escape{n}\escape{t}YOU choose}''.}}}
        \label{fig: ex02}
        
\end{subfigure}\hfill
\begin{subfigure}[t]{0.45\textwidth}
\centering
    \includegraphics[width=\linewidth]{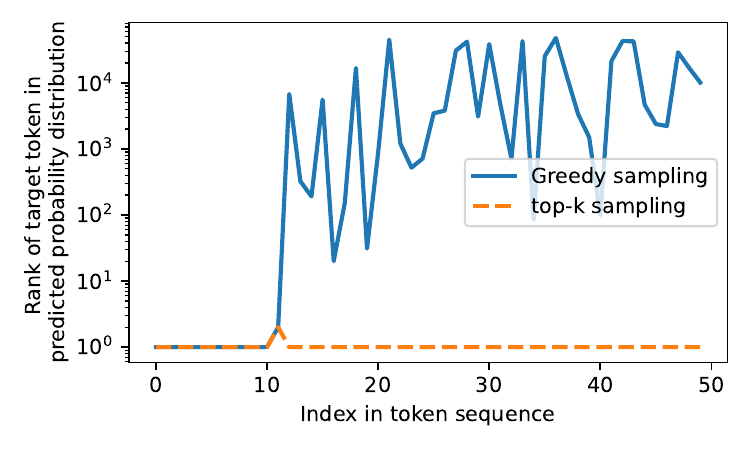}
        \caption{
        {\footnotesize
        \textbf{Prefix: }\textit{``SHIVELY, HUNTER,\escape{n} \escape{n}The PEP system closes on Friday, May 25, 2001 \escape{n} \escape{n}Our records indicate that you have been requested to provide feedback on one or more Enron employees.  The deadline for completing feedback is Friday''}.
        \textbf{Suffix (predicted from greedy sampling): } \textit{`` ,  May 25th.   \escape{n} \escape{n}Below is {\color{carminered}some information which will assist you in completing your feedback forms and email them to us at feedback@pep.enron.com.  Please note that you can add additional people within the PEP''}}. \textbf{Target Suffix: } \textit{`` ,  May 25th.   \escape{n} \escape{n}Below is {\color{greenncs}a list of feedback requests with a status of "OPEN".  Please complete or decline these requests as soon as possible by logging into PEP at http://pep.enron.com and selecting}''.}}}
        \label{fig: ex03}
\end{subfigure}
\caption{Four more examples from the Enron dataset of failures of greedy sampling to measure memorization with discoverable extraction (we give another in \Cref{fig: greedy_fail}). We highlight the differences between {\color{carminered} predicted} and {\color{greenncs} target} tokens.}
\label{fig: examples}
\end{figure*}

\section{Large models memorize more: experiments with more model sizes}\label{sec:app_more_model_sizes}

We plot more model sizes in \Cref{fig: app_model_sizes}.
Across most choices of $n$ and $p$, we find that when model parameters double, so do extraction rates, approximately.

\begin{figure*}[t]
\captionsetup[subfigure]{justification=centering}
  \centering
\begin{subfigure}[t]{0.45\textwidth}
\centering
    \includegraphics[width=1.\linewidth]{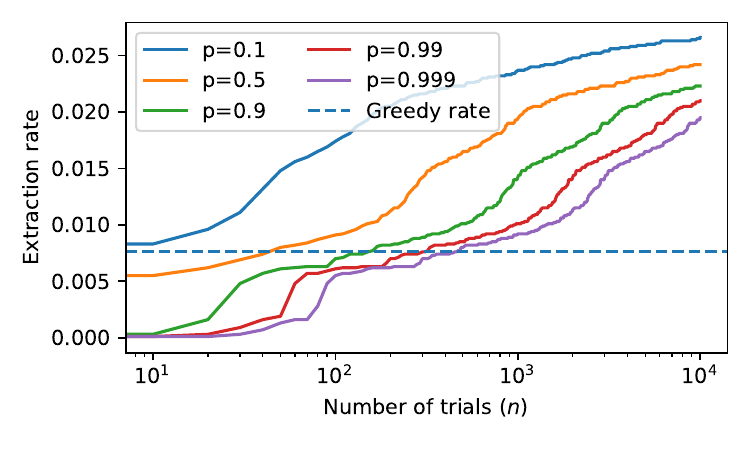}
        \caption{1B.}
        \label{fig: app_topk1b}
\end{subfigure}%
\begin{subfigure}[t]{0.45\textwidth}
\centering
    \includegraphics[width=1.\linewidth]{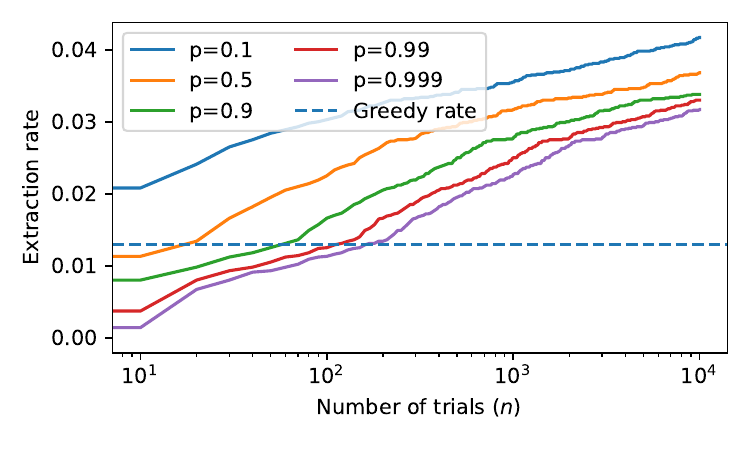}
        \caption{2.8B.}
        \label{fig: app_topk2b_notmain}
\end{subfigure}
\begin{subfigure}[t]{0.45\textwidth}
\centering
    \includegraphics[width=1.\linewidth]{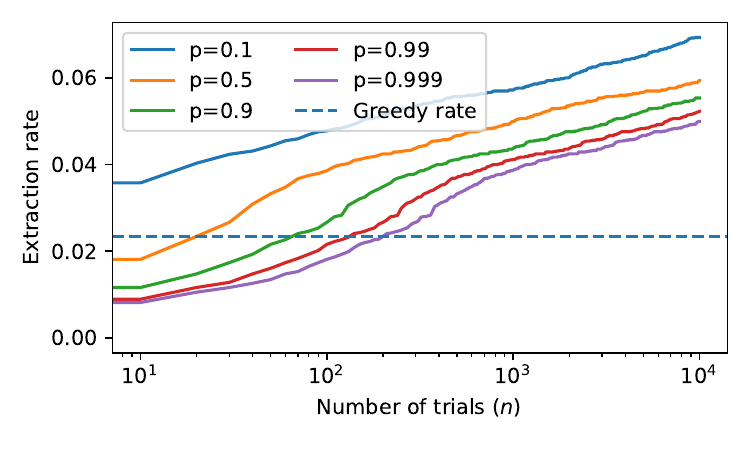}
        \caption{6.9B.}
        \label{fig: app_topk6b}
\end{subfigure}%
\begin{subfigure}[t]{0.45\textwidth}
\centering
    \includegraphics[width=1.\linewidth]{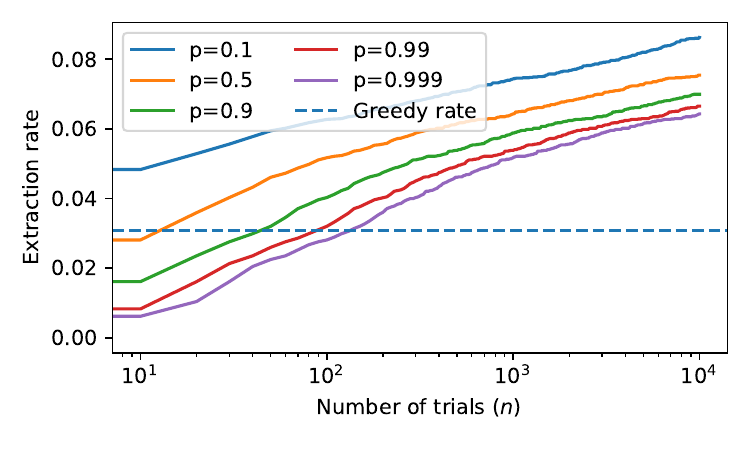}
        \caption{12B.}
        \label{fig: app_topk12b}
\end{subfigure}%
\caption{$(n, p)$-discoverable extraction for different (Pythia) model sizes using top-$k=40$ sampling.}
\label{fig: app_model_sizes}
\end{figure*}
