# Supplementary material for: Measuring memorization in language models via probabilistic extraction
Source: arXiv:2410.19482 source file (2025-03-20)
Supplement: Supplementary file 2 [file 995-appendix-repetitions.tex]

\clearpage
\section{Extraction rates for repeated training data}\label{sec: nonlog_rep}
\textcolor{red}{TODO: edits}

\begin{figure}[htbp!]
  \centering
    \includegraphics[width=.6\linewidth]{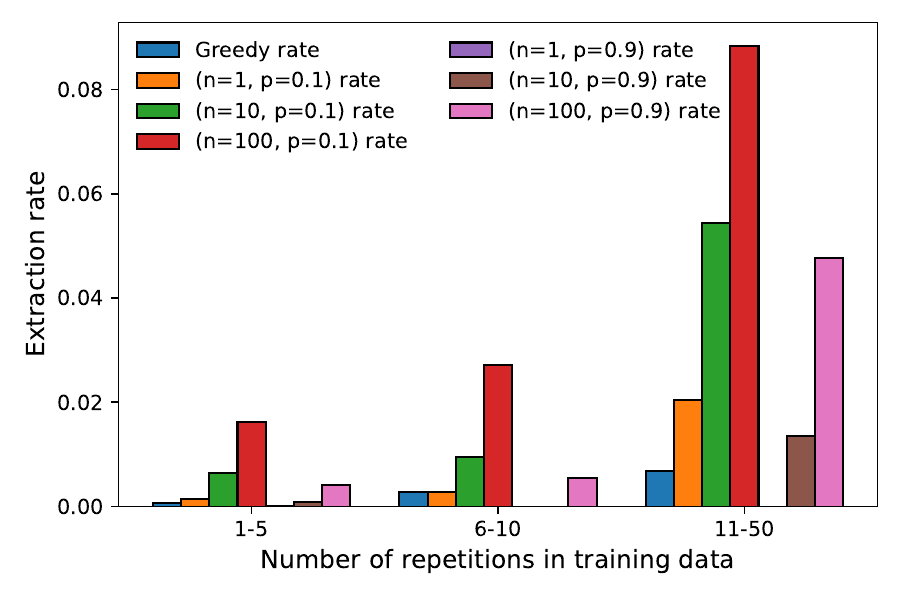}
  \caption{We plot a non log scale version of \Cref{fig: topk2b_rep_data} to make it clear that the difference between the greedy sampling extraction rate and $(n, p)$ rate increases with more training data repetitions.}
\label{fig: topk2b_rep_data_no_log}
\end{figure}

% \begin{wrapfigure}{r}{0.5\textwidth}
%   \begin{center}
% \includegraphics[width=0.5\textwidth]{figures/empirical_p.pdf}
%   \end{center}
%   \caption{We check that generating a set of $n$ sequences and checking the probability a training example appears at least once in the set (empirical $p$), matches the theoretical $p$ according to \Cref{eq:npmem}.}
%   \label{fig: emp_p}
% \end{wrapfigure}
\FloatBarrier
